# Supplementary material for: Wurtzite Phonons and the Mobility of a GaN/AlN 2D Hole Gas
Source: arXiv:1906.04947 ancillary file (2019-06-12)
Supplement: Supplementary file 1 [file Bader2019_Mobility_Supplement_arXiv.pdf]

The following article has been accepted by Applied Physics Letters.
After it is published, it will be found at https://aip.scitation.org/journal/apl

# Supplement to "Wurtzite Phonons and the Mobility of a GaN/AlN 2D Hole Gas"

## S1) Multiband kp model

The Multiband k.p matrix differential equation[1] can be split into four terms by the order of derivatives

$$\left[C^0(z) - iC^L(z)\partial_z - i\partial_z C^R(z) - \partial_z C^2(z)\partial_z\right] f(z) = \lambda f(z) \tag{S1}$$

where, for a wurtzite valence band $f(z)$ is a six-component spinor. In the basis $|X\uparrow\rangle, |Y\uparrow\rangle, |Z\uparrow\rangle, |X\downarrow\rangle, |Y\downarrow\rangle, |Z\downarrow\rangle$, these position-dependent matrices can be written

$$C^0 = C^{0L} + C^{0D} + C^{0S} \tag{S2}$$

$$C^{0L} = I_2 \otimes \begin{pmatrix} k_x L_1^u k_x + k_y M_1^u k_y & k_x N_1^+ k_y + k_y N_1^- k_x & \cdot \\ k_y N_1^+ k_x + k_x N_1^- k_y & k_x M_1^u k_x + k_y L_1^u k_y & \cdot \\ \cdot & \cdot & k_x M_3^u k_x + k_y M_3^u k_y \end{pmatrix} \tag{S3}$$

$$C^{0D} = \begin{pmatrix} \Delta_1 & -i\Delta_2 & \cdot & \cdot & \cdot & \Delta_3 \\ i\Delta_2 & \Delta_1 & \cdot & \cdot & \cdot & -i\Delta_3 \\ \cdot & \cdot & \cdot & -\Delta_3 & i\Delta_3 & \cdot \\ \cdot & \cdot & -\Delta_3 & \Delta_1 & i\Delta_2 & \cdot \\ \cdot & \cdot & -i\Delta_3 & -i\Delta_2 & \Delta_1 & \cdot \\ \Delta_3 & i\Delta_3 & \cdot & \cdot & \cdot & \cdot \end{pmatrix} \tag{S4}$$

$$C^{0S} = \begin{pmatrix} l_1 e_{xx} + m_1 e_{yy} + m_2 e_{zz} & n_1 e_{xy} & n_2 e_{xz} \\ n_1 e_{xy} & m_1 e_{xx} + l_1 e_{yy} + m_2 e_{zz} & n_2 e_{yz} \\ n_2 e_{xz} & n_2 e_{yz} & m_3 e_{xx} + m_3 e_{yy} + l_2 e_{zz} \end{pmatrix} \tag{S5}$$

$$C^L = I_2 \otimes \begin{pmatrix} \cdot & \cdot & k_x N_2^+ \\ \cdot & \cdot & k_y N_2^+ \\ k_x N_2^- & k_y N_2^- & \cdot \end{pmatrix} \tag{S6}$$

$$C^R = I_2 \otimes \begin{pmatrix} \cdot & \cdot & N_2^- k_x \\ \cdot & \cdot & N_2^- k_y \\ N_2^+ k_x & N_2^+ k_y & \cdot \end{pmatrix} \tag{S7}$$

The following article has been accepted by Applied Physics Letters.
After it is published, it will be found at https://aip.scitation.org/journal/apl

$$C^2 = I_2 \otimes \begin{pmatrix} M_2^u & \cdot & \cdot \\ \cdot & M_2^u & \cdot \\ \cdot & \cdot & L_2^u \end{pmatrix} \tag{S8}$$

where $I_2$ is the 2x2 identity matrix,

$$L_1^u = A_2 + A_4 + A_5, \quad L_2^u = A_1$$
$$M_1^u = A_2 + A_4 - A_5, \quad M_2^u = A_1 + A_3, \quad M_3^u = A_2$$
$$N_1^+ = 3A_5 - A_2 - A_4 + U; \quad N_1^- = -A_5 + A_2 + A_4 - U$$
$$N_2^+ = \sqrt{2}A_6 - A_1 - A_3 + U, \quad N_2^- = A_1 + A_3 - U$$

with $U = \frac{\hbar^2}{2m_e}$ and

$$l_1 = D_2 + D_4 + D_5, \quad l_2 = D_1$$
$$m_1 = D_2 + D_4 - D_5, \quad m_2 = D_1 + D_3, \quad m_3 = D_2$$
$$n_1 = 2D_5, \quad n_2 = \sqrt{2}D_6$$

where $A_i$ are the Rashba-Sheka-Pikus parameters and $D_i$ are the deformation potentials. Notes:

- The $A_7$ parameter is neglected as is common in heterostructural multi-band kp analysis[1]. The effects of this negligence are known[8]
- Since none of the important scattering mechanisms interact with spin and the spin-splitting is a small energy scale in the band structure, one can "cheat" that degree of freedom to speed up calculations. For faster evaluation of mobility, the off-diagonal 3x3 blocks of $C_{0D}$ are zeroed and a sub-meV up-down term is added along the diagonal to ensure the spins have a finite non-degeneracy. Then the mobility calculation can account for only one of the spins and assume the same for the other.
- The above calculation is a 6x6 kp method in which the valence bands are accounted for directly and the conduction band appears only as a perturbation. Since GaN is a wide-bandgap material, this convenient simplification is reasonably accurate as compared to a slower 8x8 kp implementation.

# S2) Acoustic phonon dispersion

As given in the main text, the elastic continuum model joins the continuum Newton's law with the material stress-strain relation[7]:

$$\rho \frac{\partial^2 u_i}{\partial t^2} = \frac{\partial T_{ij}}{\partial r_j}, \quad T_{ij} = c_{ijkl}\epsilon_{kl} \tag{S9}$$

The following article has been accepted by Applied Physics Letters.
After it is published, it will be found at https://aip.scitation.org/journal/apl

where $u_i$ is the local displacement, $\rho$ is the density, $T_{ij}$ is the stress tensor, $c_{ijkl}$ is the stiffness tensor, and $\epsilon_{ijkl}$ is the strain tensor $\epsilon_{ij} = \frac{1}{2}\left(\partial_{r_j} u_i + \partial_{r_i} u_j\right)$. The latter equation can be re-expressed in Voigt notation

$$T_\alpha = c_{\alpha\beta}\epsilon_\beta \tag{S10}$$

where $\alpha, \beta$ run 1-6 and the Voigt tuples are related to the actual tensors by

$$T_1 = T_{xx}, \quad \epsilon_1 = \epsilon_{xx} \tag{S11}$$
$$T_2 = T_{yy}, \quad \epsilon_2 = \epsilon_{yy} \tag{S12}$$
$$T_3 = T_{zz}, \quad \epsilon_3 = \epsilon_{zz} \tag{S13}$$
$$T_4 = T_{yz}, \quad \epsilon_4 = 2\epsilon_{yz} \tag{S14}$$
$$T_5 = T_{xz}, \quad \epsilon_5 = 2\epsilon_{xz} \tag{S15}$$
$$T_6 = T_{xy}, \quad \epsilon_6 = 2\epsilon_{xy} \tag{S16}$$

For a wurtzite crystal, the $c_{\alpha\beta}$ can be written

$$c = \begin{pmatrix} C_{11} & C_{12} & C_{13} & 0 & 0 & 0 \\ C_{12} & C_{22} & C_{13} & 0 & 0 & 0 \\ C_{13} & C_{13} & C_{33} & 0 & 0 & 0 \\ 0 & 0 & 0 & C_{44} & 0 & 0 \\ 0 & 0 & 0 & 0 & C_{44} & 0 \\ 0 & 0 & 0 & 0 & 0 & \frac{1}{2}\left(C_{11} - C_{12}\right) \end{pmatrix} \tag{S17}$$

For a wurtzite structure uniform in the basal plane but possibly inhomogenous along $z$, we note that the elastic continuum model is rotationally symmetric in plane, so we can choose the in-plane wavevector along $x$ and assume phonons have a form

$$u = \begin{pmatrix} u_x(z) \\ u_y(z) \\ u_z(z) \end{pmatrix} e^{i(qx-\omega t)} \tag{S18}$$

We will hide the explicit $z$ dependence for now. The the strain can be evaluated

$$\epsilon_1 = iqu_x, \qquad \epsilon_4 = \partial_z u_y \tag{S19}$$
$$\epsilon_2 = 0, \qquad \epsilon_5 = iqu_z + \partial_z u_x \tag{S20}$$
$$\epsilon_3 = \partial_z u_z, \qquad \epsilon_6 = iqu_y \tag{S21}$$

Then the two constitutive laws can be combined as

$$-\rho\omega^2 \begin{pmatrix} u_x \\ u_y \\ u_z \end{pmatrix} = \begin{pmatrix} -C_{11}q^2 u_x + iqC_{13}\partial_z u_z + \partial_z C_{44} iqu_z + \partial_z C_{44}\partial_z u_x \\ -\frac{1}{2}\left(C_{11} - C_{12}\right) q^2 u_y + \partial_z C_{44}\partial_z u_y \\ -C_{44}q^2 u_z + C_{44} iq\partial_z u_x + iq\partial_z C_{13} u_x + \partial_z C_{33}\partial_z u_z \end{pmatrix} \tag{S22}$$

This matrix can be split by order

$$\rho\omega^2 u = Cu, \quad C = q^2 C^0 - iqC^L\partial_z - iq\partial_z C^R - \partial_z C^2 \partial_z \tag{S23}$$

The following article has been accepted by Applied Physics Letters.
After it is published, it will be found at https://aip.scitation.org/journal/apl

where

$$C^0 = \begin{pmatrix} C_{11} & & \\ & \frac{1}{2}(C_{11} - C_{12}) & \\ & & C_{44} \end{pmatrix}, \quad C^2 = \begin{pmatrix} C_{44} & & \\ & C_{44} & \\ & & C_{33} \end{pmatrix} \tag{S24}$$

$$C^L = \begin{pmatrix} & & C_{13} \\ & 0 & \\ C_{44} & & \end{pmatrix}, \quad C^R = \begin{pmatrix} & & C_{44} \\ & 0 & \\ C_{13} & & \end{pmatrix} \tag{S25}$$

This generalized eigenvalue problem can be solved by the Finite Element Method once boundary conditions are prescribed. Specifically, the upper boundary will be treated as free to vibrate (*i.e.* Neumann), so $T_{iz} = 0$. The bottom boundary is unimportant in the limit of a thick buffer, but, to preclude the appearance of an irrelevant bottom-boundary mode decaying upwards into AlN, one may set the bottom boundary by Dirichelet $u_i = 0$ condition.

We note here that in the above matrices, there is no coupling between the Y (second) component and the XZ (first and third) components, so the problem could be further broken apart into a pair of problems if desired.

## S2.1) Piezoelectric potential

Once the acoustic phonon modes are solved for, each mode can be considered a source of piezoelectric charge, which induces a further scattering potential. This approximation of treating the acoustic and electric problem separately is common practice[6] given the low-frequency of zone-center acoustic phonons. A phonon in a piezoelectric material induces a charge

$$\rho = -\nabla \cdot \vec{P} = -\nabla \cdot \left[ \begin{pmatrix} 0 & 0 & 0 & 0 & e_{15} & 0 \\ 0 & 0 & 0 & e_{15} & 0 & 0 \\ e_{31} & e_{31} & e_{33} & 0 & 0 & 0 \end{pmatrix} \begin{pmatrix} \epsilon_{xx} \\ \epsilon_{yy} \\ \epsilon_{zz} \\ 2\epsilon_{yz} \\ 2\epsilon_{xz} \\ 2\epsilon_{xy} \end{pmatrix} \right] \tag{S26}$$

where $e_{\alpha\beta}$ are the piezoelastic moduli

$$= -\nabla \cdot \begin{pmatrix} e_{15}\epsilon_{xz} \\ e_{15}\epsilon_{yz} \\ e_{31}\epsilon_{xx} + e_{31}\epsilon_{yy} + e_{33}\epsilon_{zz} \end{pmatrix} \tag{S27}$$

$$= -e_{15}(iq_x\epsilon_{xz} + iq_y\epsilon_{yz}) - \partial_z[e_{31}(\epsilon_{xx} + \epsilon_{yy}) + e_{33}\epsilon_{zz}] \tag{S28}$$

$$= -e_{15}(iq_x\partial_z u_x - q_x^2 u_z + iq_y\partial_z u_y - q_y^2 u_z) \tag{S29}$$

$$- \partial_z[ie_{31}(q_x u_x + q_y u_y) + e_{33}\partial_z u_z] \tag{S30}$$

$$= -e_{15}(iq\partial_z u_L - q^2 u_z) - \partial_z[iqe_{31}u_L + e_{33}\partial_z u_z] \tag{S31}$$

$$= q^2 e_{15} u_z - iqe_{15}\partial_z u_L - iq\partial_z e_{31} u_L - \partial_z e_{33}\partial_z u_z \tag{S32}$$

where $u_L$ is the in-plane longitudinal component of the displacement. Plugging this into the Poisson equation, we find a potential

$$-\nabla\left[\varepsilon\nabla\phi\right]=\rho \tag{S33}$$

$$q^2\varepsilon_\perp\phi-\partial_z\varepsilon_\parallel\partial_z\phi=\rho \tag{S34}$$

So

$$q^2\varepsilon_\perp\phi-\partial_z\varepsilon_\parallel\partial_z\phi=q^2e_{15}u_z-iqe_{15}\partial_z u_L-iq\partial_z e_{31}u_L-\partial_z e_{33}\partial_z u_z \tag{S35}$$

which can be written

$$C^0\phi-\partial_z C^2\partial_z\phi=C^{0'}u_z-iC^{L'}\partial_z u_x-i\partial_z C^{R'}u_x-\partial_z C^{2'}\partial_z u_z \tag{S36}$$

where

$$C_0=q^2\varepsilon_\perp,\quad C_2=\varepsilon_\parallel \tag{S37}$$

$$C^{0'}=q^2e_{15},C^{L'}=qe_{15},C^{R'}=qe_{31},C^{2'}=e_{33} \tag{S38}$$

and solved by the Finite Element Method.

# S3) Polar optical phonon dispersion

As discussed in the main text, the interaction of the uniaxial polar atomic lattice with electromagnetic waves can be incorporated as a pair of frequency-dependent dielectric constants $\varepsilon_\parallel$ and $\varepsilon_\perp$, upon which solving the Poisson equation gives all the modes which produce an electric potential [that is, all the modes which are important for POP scattering]. For in-plane wavevector $q$,

$$\partial_z\epsilon_\parallel\partial_z\phi=q^2\epsilon_\perp\phi \tag{S39}$$

The normalization condition given in the main text, applied to both classes of phonon, is expressed in terms of $u$, but, by solving for $u$ as a function of $\phi$, this condition can be re-expressed directly in terms of $\phi$:

$$\frac{\hbar}{2\omega}=\int dz\varepsilon_\infty(\omega_{LO}^2-\omega_{TO}^2)\left(\left(\frac{\partial_z\phi}{\omega_{TO\parallel}^2-\omega^2}\right)^2+\left(\frac{q\phi}{\omega_{TO\perp}^2-\omega^2}\right)^2\right) \tag{S40}$$

Given the frequency-dependence of the parameters in the equation, a numerical solution of the eigenvalue problem is actually somewhat involved. Fortunately, the discretely layered binary heterostructure structure lends itself to analytic solutions. We will solve a single heterojunction structure 1/2 where materials 1 and 2 are GaN or AlN in either order, and the bottom material is semi-infinite. The top surface at $z=0$ is assumed Dirichelet. The thickness of the top layer is $t_1$ and a normalization thickness of $t_2$ is set for the bottom layer which will discretize the bottom-region-confined states.

In a given region, solutions are oscillating if $\varepsilon_\perp\varepsilon_\parallel < 0$ and exponential if $\varepsilon_\perp\varepsilon_\parallel > 0$. At an interface, the derivative switches signs iff $\varepsilon_{1\parallel}\varepsilon_{2\parallel} < 0$. We will use the following convenient definitions, similar to the notation of Komirenko[5] but for a factor of two in $\alpha$

$$\xi_i = \sqrt{|\varepsilon_{i\perp}\varepsilon_{i\parallel}|}, \quad \alpha_i = \sqrt{|\varepsilon_{i\perp}/\varepsilon_{i\parallel}|} \tag{S41}$$

Then the vertical wavevector of a mode in a given region is $k_i = q\alpha_i$.

If the solution is written in Region 1 with some normalization constant $A$ and Region 2 with some normalization constant $B$, then the first matching condition $\phi(t_1^-) = \phi_2(t_1^+)$ gives us some expression for $B/A$, and the normalization condition will be written for $A$:

$$A^2 = \frac{\hbar}{2\omega}\Big/\left[\beta_{\parallel 1}^2\gamma_{\parallel 1}^2 + \beta_{\perp 1}^2\gamma_{\perp 1}^2 + \left(\frac{B}{A}\right)^2\left(\beta_{\parallel 2}^2\gamma_{\parallel 2}^2 + \beta_{\perp 2}^2\gamma_{\perp 2}^2\right)\right] \tag{S42}$$

with

$$\beta_{\parallel i}^2 = \varepsilon_i^\infty\left(\omega_{LOi}^2 - \omega_{TOi}^2\right)\left(\frac{k_i}{\omega_{TO\parallel i}^2 - \omega^2}\right)^2 \tag{S43}$$

$$\beta_{\perp i}^2 = \varepsilon_i^\infty\left(\omega_{LOi}^2 - \omega_{TOi}^2\right)\left(\frac{q}{\omega_{TO\perp i}^2 - \omega^2}\right)^2 \tag{S44}$$

and

$$\gamma_{\parallel i}^2 = \int_i dz\left(\frac{\partial_z\phi}{Ak_i}\right)^2, \quad \gamma_{\perp i}^2 = \int_i dz\left(\frac{\phi}{B}\right)^2 \tag{S45}$$

From there on out, the solution is a simple mechanical procedure, depending on the signs of the dielectric constants.

## S3.1) Confined to Region 1

If the solution is oscillating in Region 1 and decaying in Region 2, we can write

$$\phi_1 = A\sin(k_1 z), \quad \phi_2 = Be^{-k_2 z} \tag{S46}$$

Matching interface conditions gives

$$q = \frac{1}{\alpha_1 t_1}\left[\tan^{-1}(\xi_1/\xi_2) + \pi n\right] \tag{S47}$$

with $B/A = \sin(k_1 t_1)e^{k_2 t_1}$ and

$$\gamma_{\parallel 1} = \frac{1}{2}(t_1 + \frac{1}{2k_1}\sin(2k_1 t_1)), \quad \gamma_{\perp 1} = \frac{1}{2}(t_1 - \frac{1}{2k_1}\sin(2k_1 t_1)) \tag{S48}$$

$$\gamma_{\parallel 2} = \frac{1}{2k_2}e^{-2k_2 t_1}, \quad \gamma_{\perp 2} = \frac{1}{2k_2}e^{-2k_2 t_1} \tag{S49}$$

### S3.2) Confined to Interface

If the solution is decaying in both regions, we can write

$$\phi_1 = A\sinh(k_1 z), \quad \phi_2 = Be^{-k_2 z} \tag{S50}$$

Matching interface conditions gives

$$q = \frac{1}{2\alpha t_1}\log\left[\frac{\xi_2+\xi_1}{\xi_2-\xi_1}\right] \tag{S51}$$

with $B/A = \sinh(k_1 t_1)e^{k_2 t_1}$ and

$$\gamma_{\parallel 1} = \frac{1}{2}\left(\frac{1}{2k_1}\sinh(2k_1 t_1) + t_1\right), \quad \gamma_{\perp 1} = \frac{1}{2}\left(\frac{1}{2k_1}\sinh(2k_1 t_1) - t_1\right) \tag{S52}$$

$$\gamma_{\parallel 2} = \frac{1}{2k_2}e^{-2k_2 t_1}, \quad \gamma_{\perp 2} = \frac{1}{2k_2}e^{-2k_2 t_1} \tag{S53}$$

### S3.3) Confined to Region 2

If the solution is decaying in Region 1 and oscillating in Region 2, we can write

$$\phi_1 = A\sinh(k_1 z), \quad \phi_2 = B\sin(k_2 z + \theta) \tag{S54}$$

Matching interface conditions gives

$$\theta = \tan^{-1}\left(\frac{\xi_2}{\xi_1}\tanh(k_1 t_1)\right) - k_2 t_1 \tag{S55}$$

with $B/A = \sinh(k_1 t_1)/\sin(k_2 t_1 + \theta)$. The $t_2$ thickness normalization gives $k_2 = \pi(n+1)/t_2$, so

$$q = \frac{\pi(n+1)}{\alpha_2 t_2} \tag{S56}$$

Normalization is accounted for via

$$\gamma_{\parallel 1} = \frac{1}{2}\left(\frac{1}{2k_1}\sinh(2k_1 t_1) + t_1\right), \quad \gamma_{\perp 1} = \frac{1}{2}\left(\frac{1}{2k_1}\sinh(2k_1 t_1) - t_1\right) \tag{S57}$$

$$\gamma_{\parallel 2} = \frac{t_2}{2}, \quad \gamma_{\perp 2} = \frac{t_2}{2} \tag{S58}$$

## S4) Numerical details

Most material parameters are drawn from Vurgaftman and Meyer's compilation[11], but anisotropic dielectric constants are from the measurements of Kane[3] and Kazan[4], optical phonon parameters are from the compilation in Komirenko[5] and the polarization-related quantities are computed from the calculations of Dreyer[2]. To ensure that the results do not depend on the specific choice of $k \cdot p$

parameters, we performed the entire calculation with not only the $k \cdot p$ parameters from Vurgaftman and Meyer but also ran a comparison with more recent parameters fitted by Rinke[9] from atomistic GW calculations (but keeping the $\Delta_{SO}$ since Rinke neglects this). Results and trends were quite similar despite the differences in individual parameters.

The first step in each mobility point is calculation of the band diagram by a standard Newton iteration of a charge model (including analytical derivatives) and the Poisson equation (as laid out in Tan's work[10]). The Poisson equation includes a Dirichelet boundary at the surface (SBH of 1.4 eV) and a Neumann boundary at the artificial bottom termination (500nm of AlN). The charge density consists of polarization contributions (from the interface discontinuities), quantum carrier densities (from occupation of the MBKP-solved states in a region extending from the surface to several nanometers below the interface), classical carrier densities (from occupation of the band-edge DOS in a region extending from several nanometers below the interface down the rest of the domain), and a small background ($1 \times 10^{17}/\mathrm{cm}^3$) of deep donor-like defects throughout. To achieve convergence over a wide range of conditions and temperatures despite extreme charges, the algorithm begins by artificially scaling up all dielectric constants by orders of magnitude to decouple the charge and fields, and then ramps the dielectric constants to their true values. For the simulations with varied strain, the Fermi level at the surface is adjusted (mimicking application of a gate) to keep the hole sheet density at a particular set value.

Separately, the phonon energies are evaluated by the means described in the above sections, with the caveat that the artificial bottom termination for the phonon solution domain is 40nm into the AlN (rather than 500nm as used for electrical simulation). This abridgment drastically reduces the time and storage requirements of the mobility solution, mainly by reducing the number of pseudo-continuum modes which must be considered, but is deep enough that the artificial confinement effects on the phonon spectra are at an energy scale well below thermal energy over the entire temperature range where phonons contribute significantly to scattering. Specifically, the phonon states used are the first 400 acoustic modes (including discrete and pseudo-continuum states indiscriminately), the first 20 AlN-confined optical modes of each polarization, the first 30 GaN-confined modes of each polarization, and both polarizations of the interface optical mode.

With both phonon and electron states solved, we then solve the Linearized Boltzmann Transport Equation. We first discretize $k$-space. In regions of $k$-space where the occupation changes rapidly with $k$ (that is, essentially, regions within a $k_bT$ scale of the Fermi energy and with significant group velocity), it is vital to define a dense grid. However, since this equation is to be solved over a wide range of temperatures and under many variations of the bandstructure, the precise locations of these important regions are not known in advance. Thus, an adaptive mesh is formed by the following procedure.

The mesh will be uniform in the $\theta$ direction, but variably spaced along $k$. The derivative $D$ of circularly averaged occupation with respect to $k$ is calculated ($D = \frac{1}{2\pi}\partial_k \int d\theta f(k,\theta)$ ), and an upper bound $k_{\max}$ for the $k$-mesh is determined

by a point beyond which $D$ has fallen off to a negligible value compared to its peak. The simplest strategy would be then to space mesh points evenly with respect to $k$ from zero to this upper bound. A more aggressive strategy is to space mesh points evenly with respect to circularly averaged occupation, thus regions with a rapidly changing occupation have the higher density of points. For this work, a compromise is struck in which the $k$-points are placed evenly along a weighted average (.7+.3) of $\frac{1}{2\pi}\int d\theta f(k,\theta)$ and $k/k_{\max}$, ensuring a spread of $k$-points which cluster around the vital regions. Employing this adaptive scheme, a relatively small grid of 25 $k$-values x 18 $\theta$ values (or, for simulations in which hexagonal symmetry broken, 25x24) was found sufficient. This is the mesh on which transition matrix elements will be calculated.

This mesh is further refined by even subdivision (here by a factor of 4) for the computation of the energy-conserving $\delta$ function factor, a more rapidly varying factor of position. For each subcell, all the other subcells into which the centerpoint of that subcell may legally scatter are found, and the delta-function determinant is computed using $k$-derivatives evaluated at the subcell centers. These contributions over subcells are then summed to produce a sparse matrix of the conservation factors between each cell of the original mesh described in the previous paragraph. Then, on the original mesh, the necessary transition matrix elements can be calculated only where needed by the relevant interaction Hamiltonian and the two factors are multiplied.

Explicitly, those transition matrix elements, the $H^l(q)$ in Eq 5 of the main text, are as follows. For acoustic phonons, $H^l = H^l_{adp} + H^l_{pz}$. $H^l_{adp} = C^{0S}(z)$ from Eq (S5) using the strain phasors $e_{ii}(z)$ from the acoustic mode of level $l$ solved for in Sec S2) and the material dependent $D_i(z)$ parameters. $H^l_{pz} = -e\phi(z)$ where $\phi$ is the piezoelectric potential generated by the acoustic mode of level $l$ as solved in Sec S2.1). For polar optical phonons, $H^l_{pop} = -e\phi(z)$ where $\phi(z)$ is the potential coupled with the POP mode of level $l$. Finally, for the "generic extrinsic scatterer", $H^l$ is just a constant (17.3 meV) tuned to fit the low-temperature mobility.

The transition rates are arranged to form a transition matrix $R^{k'm'}_{km}$, and thus Eq (4) of the main text is solved by a least squares procedure to find the perturbation-per-electric-field of the carrier distribution function, from which the mobility is extracted by an occupation-weighted sum of the group velocities.

# References

[1] Stefan Birner. "Modeling of semiconductor nanostructures and semiconductor – electrolyte interfaces". PhD thesis. Technical University of Munich, 2011. ISBN: 9783941650350.

[2] Cyrus E. Dreyer et al. "Correct implementation of polarization constants in wurtzite materials and impact on III-nitrides". In: *Phys. Rev. X* 6.2 (2016), p. 1. ISSN: 21603308. DOI: 10.1103/PhysRevX.6.021038.

The following article has been accepted by Applied Physics Letters.
After it is published, it will be found at https://aip.scitation.org/journal/apl

[3] M. J. Kane et al. “Determination of the dielectric constant of GaN in the kHz frequency range”. In: *Semiconductor Science and Technology* 26.8 (2011), p. 1. ISSN: 02681242. DOI: 10.1088/0268/26/8/085006.

[4] M. Kazan et al. “Directional dependence of AlN intrinsic complex dielectric function, optical phonon lifetimes, and decay channels measured by polarized infrared reflectivity”. In: *J. App. Phys.* 106.2 (2009). ISSN: 00218979. DOI: 10.1063/1.3177323.

[5] S. Komirenko et al. “Dispersion of polar optical phonons in wurtzite quantum wells”. In: *Phys. Rev. B* 59.7 (1999), p. 5013. ISSN: 0163. DOI: 10.1103/PhysRevB.59.5013.

[6] Evgenii P. Pokatilov, Denis L. Nika, and Alexander A. Balandin. “Confined electron-confined phonon scattering rates in wurtzite AlN/GaN/AlN heterostructures”. In: *J. App. Phys.* 95.10 (2004), p. 5626. ISSN: 00218979. DOI: 10.1063/1.1710705.

[7] Evghenii P. Pokatilov, Denis L. Nika, and Alexander A. Balandin. “Phonon spectrum and group velocities in AlN/GaN/AlN and related heterostructures”. In: *Superlattices and Microstructures* 33.3 (2003), p. 155. ISSN: 07496036. DOI: 10.1016/S0749(03)00069.

[8] G. B. Ren, Y. M. Liu, and P. Blood. “Valence-band structure of wurtzite GaN including the spin-orbit interaction”. In: *App. Phys. Letters* 74.8 (1999), p. 1117. ISSN: 00036951. DOI: 10.1063/1.123461.

[9] Patrick Rinke et al. “Consistent set of band parameters for the group-III nitrides AlN, GaN, and InN”. In: *Phys. Rev. B - Condensed Matter and Materials Physics* (2008). ISSN: 10980121. DOI: 10.1103/PhysRevB.77.075202.

[10] I-H. Tan et al. “A self-consistent solution of Schrödinger–Poisson equations using a nonuniform mesh”. In: *J. App. Phys.* 68.8 (Oct. 1990), p. 4071. ISSN: 00218979. DOI: 10.1063/1.346245.

[11] I. Vurgaftman and J. R. Meyer. “Band parameters for nitrogen-containing semiconductors”. In: *J. App. Phys.* 94.6 (2003), p. 3675. ISSN: 00218979. DOI: 10.1063/1.1600519.
